# Supplementary material for: Towards Scalable 3D Anomaly Detection and Localization: A Benchmark via 3D Anomaly Synthesis and A Self-Supervised Learning Network
Source: arXiv:2311.14897 source file (2023-11-30)
Supplement: Supplementary file 1 [file effect.tex]

% \vspace{-4mm}

% \end{figure}
\begin{figure*}
    \subfloat[Iteration number influence.]{
        \begin{minipage}[t]{0.46\linewidth}
            \centering
            \includegraphics[width=0.9\linewidth]{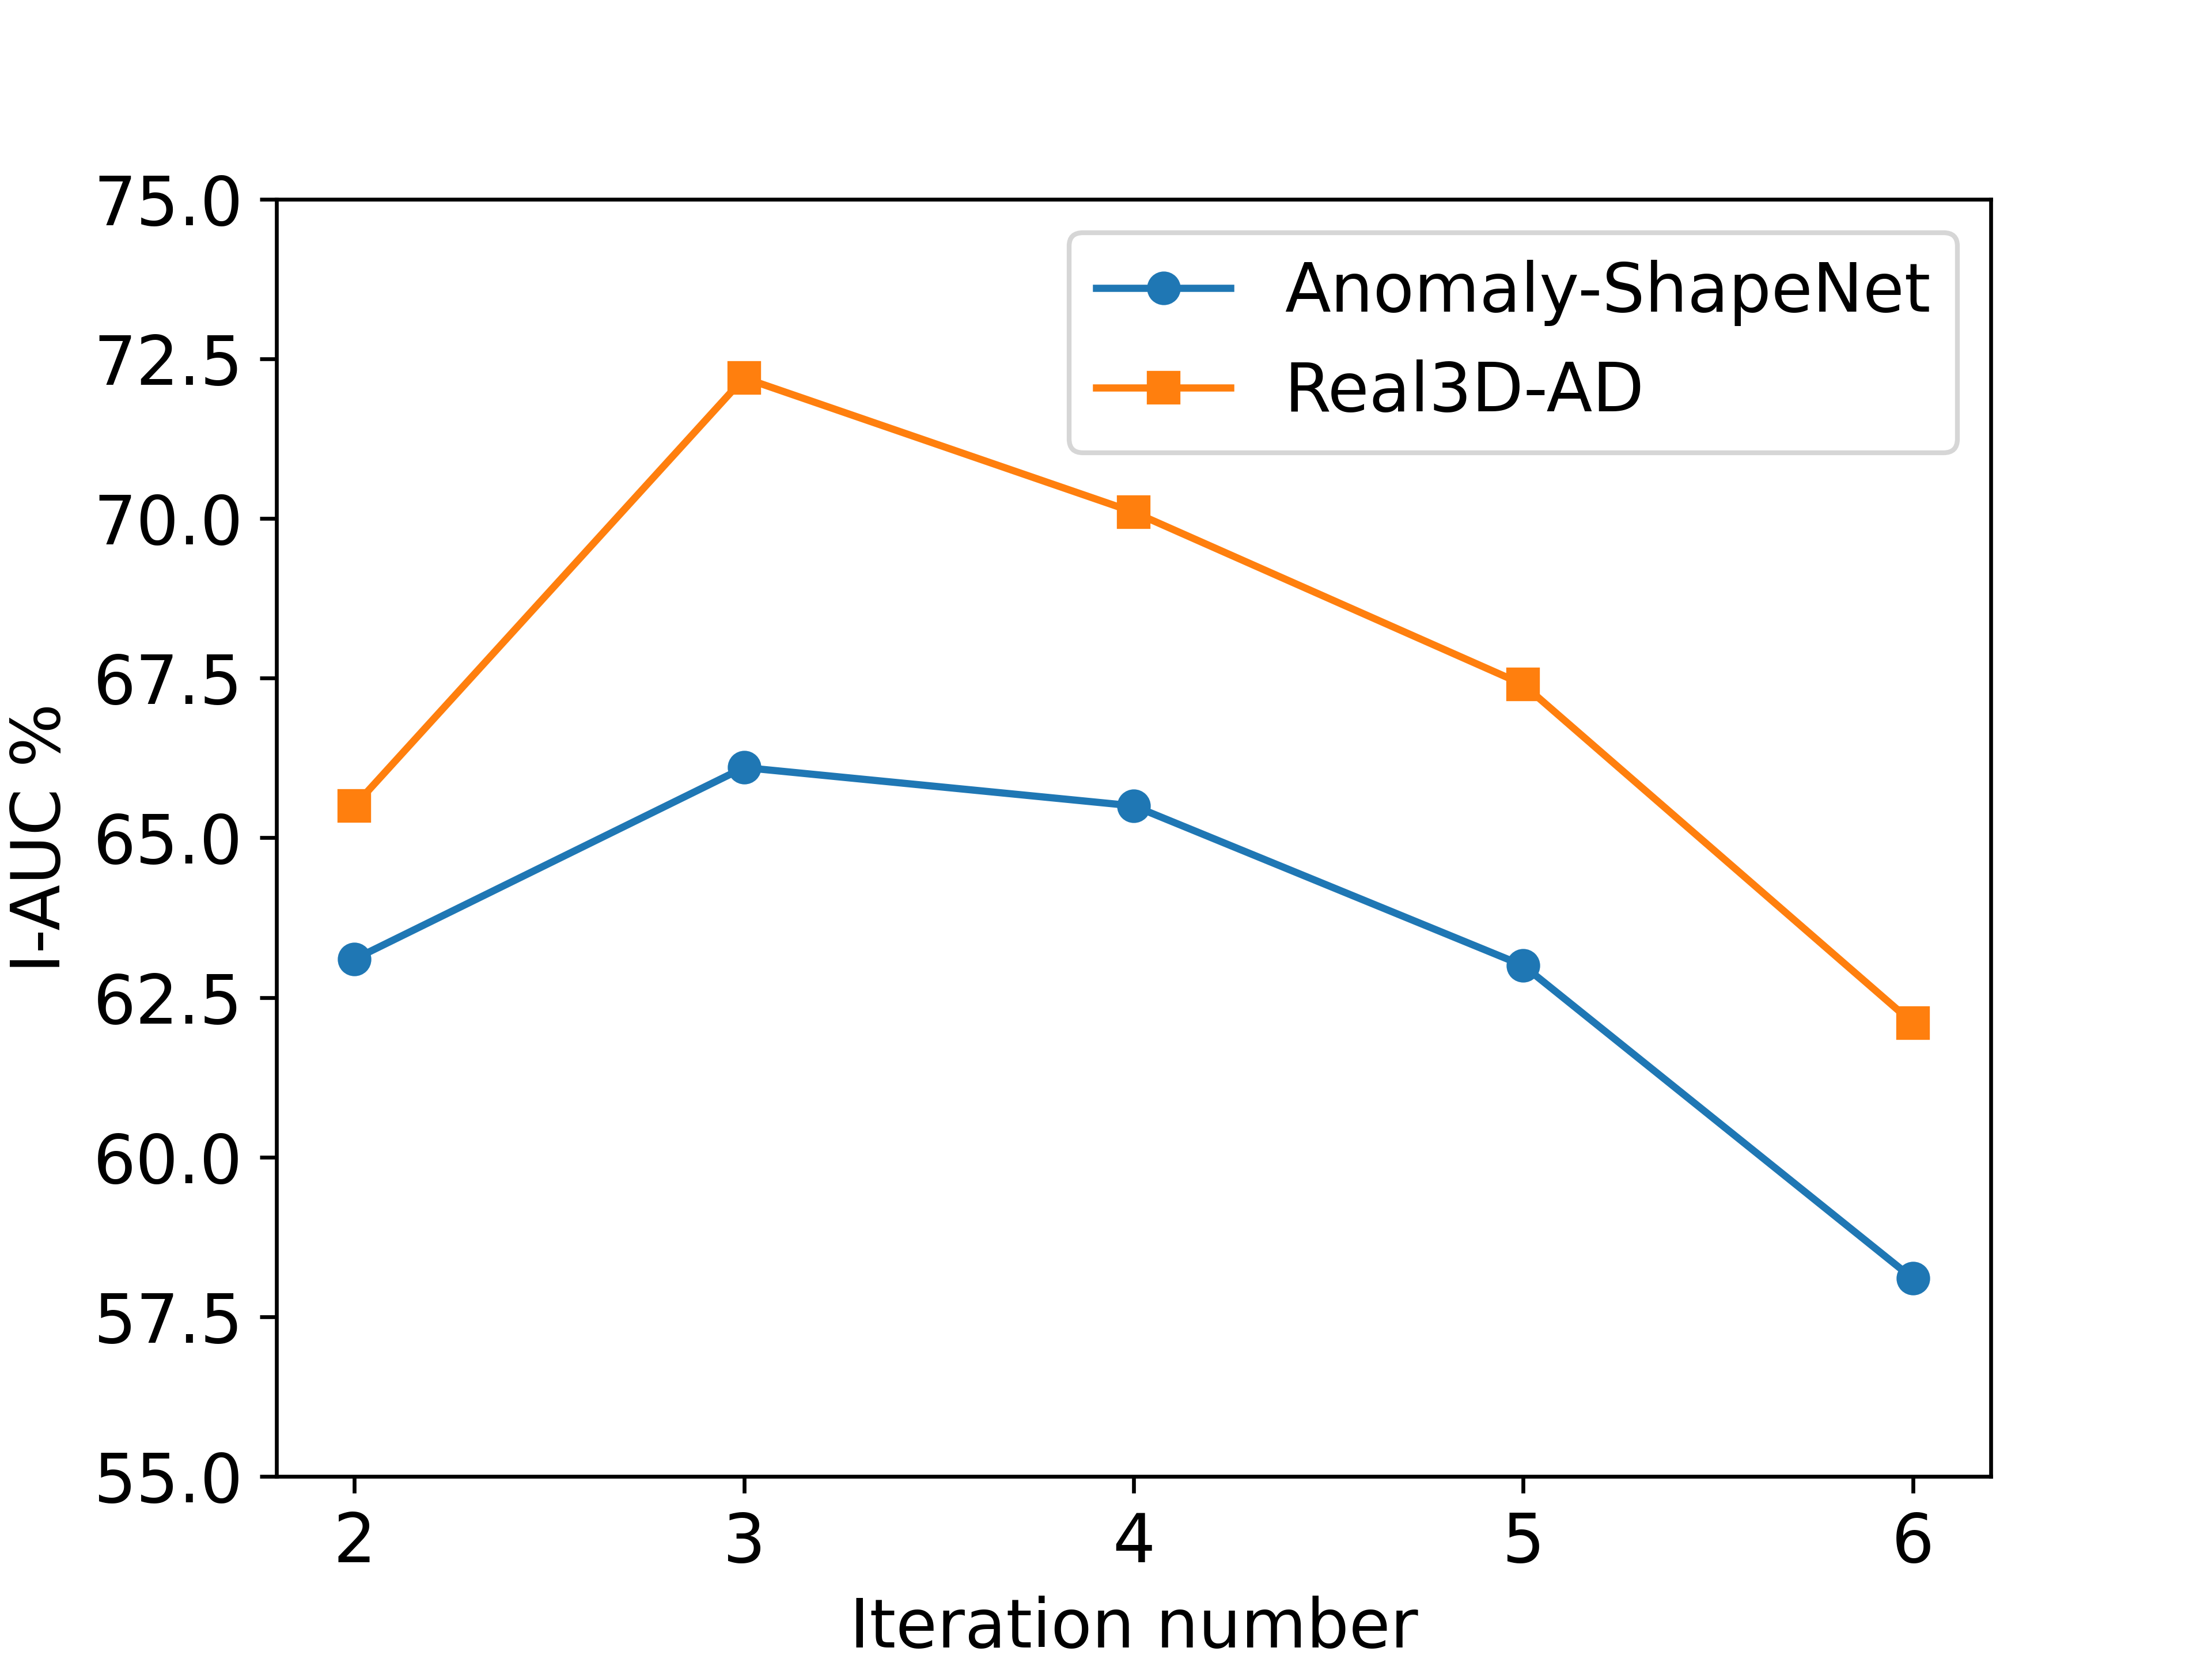}
            \label{fig:iter}
        \end{minipage}
    }
    \hfill
    \subfloat[Patch size influence.]{
        \begin{minipage}[t]{0.46\linewidth}
            \centering
            \includegraphics[width=0.9\linewidth]{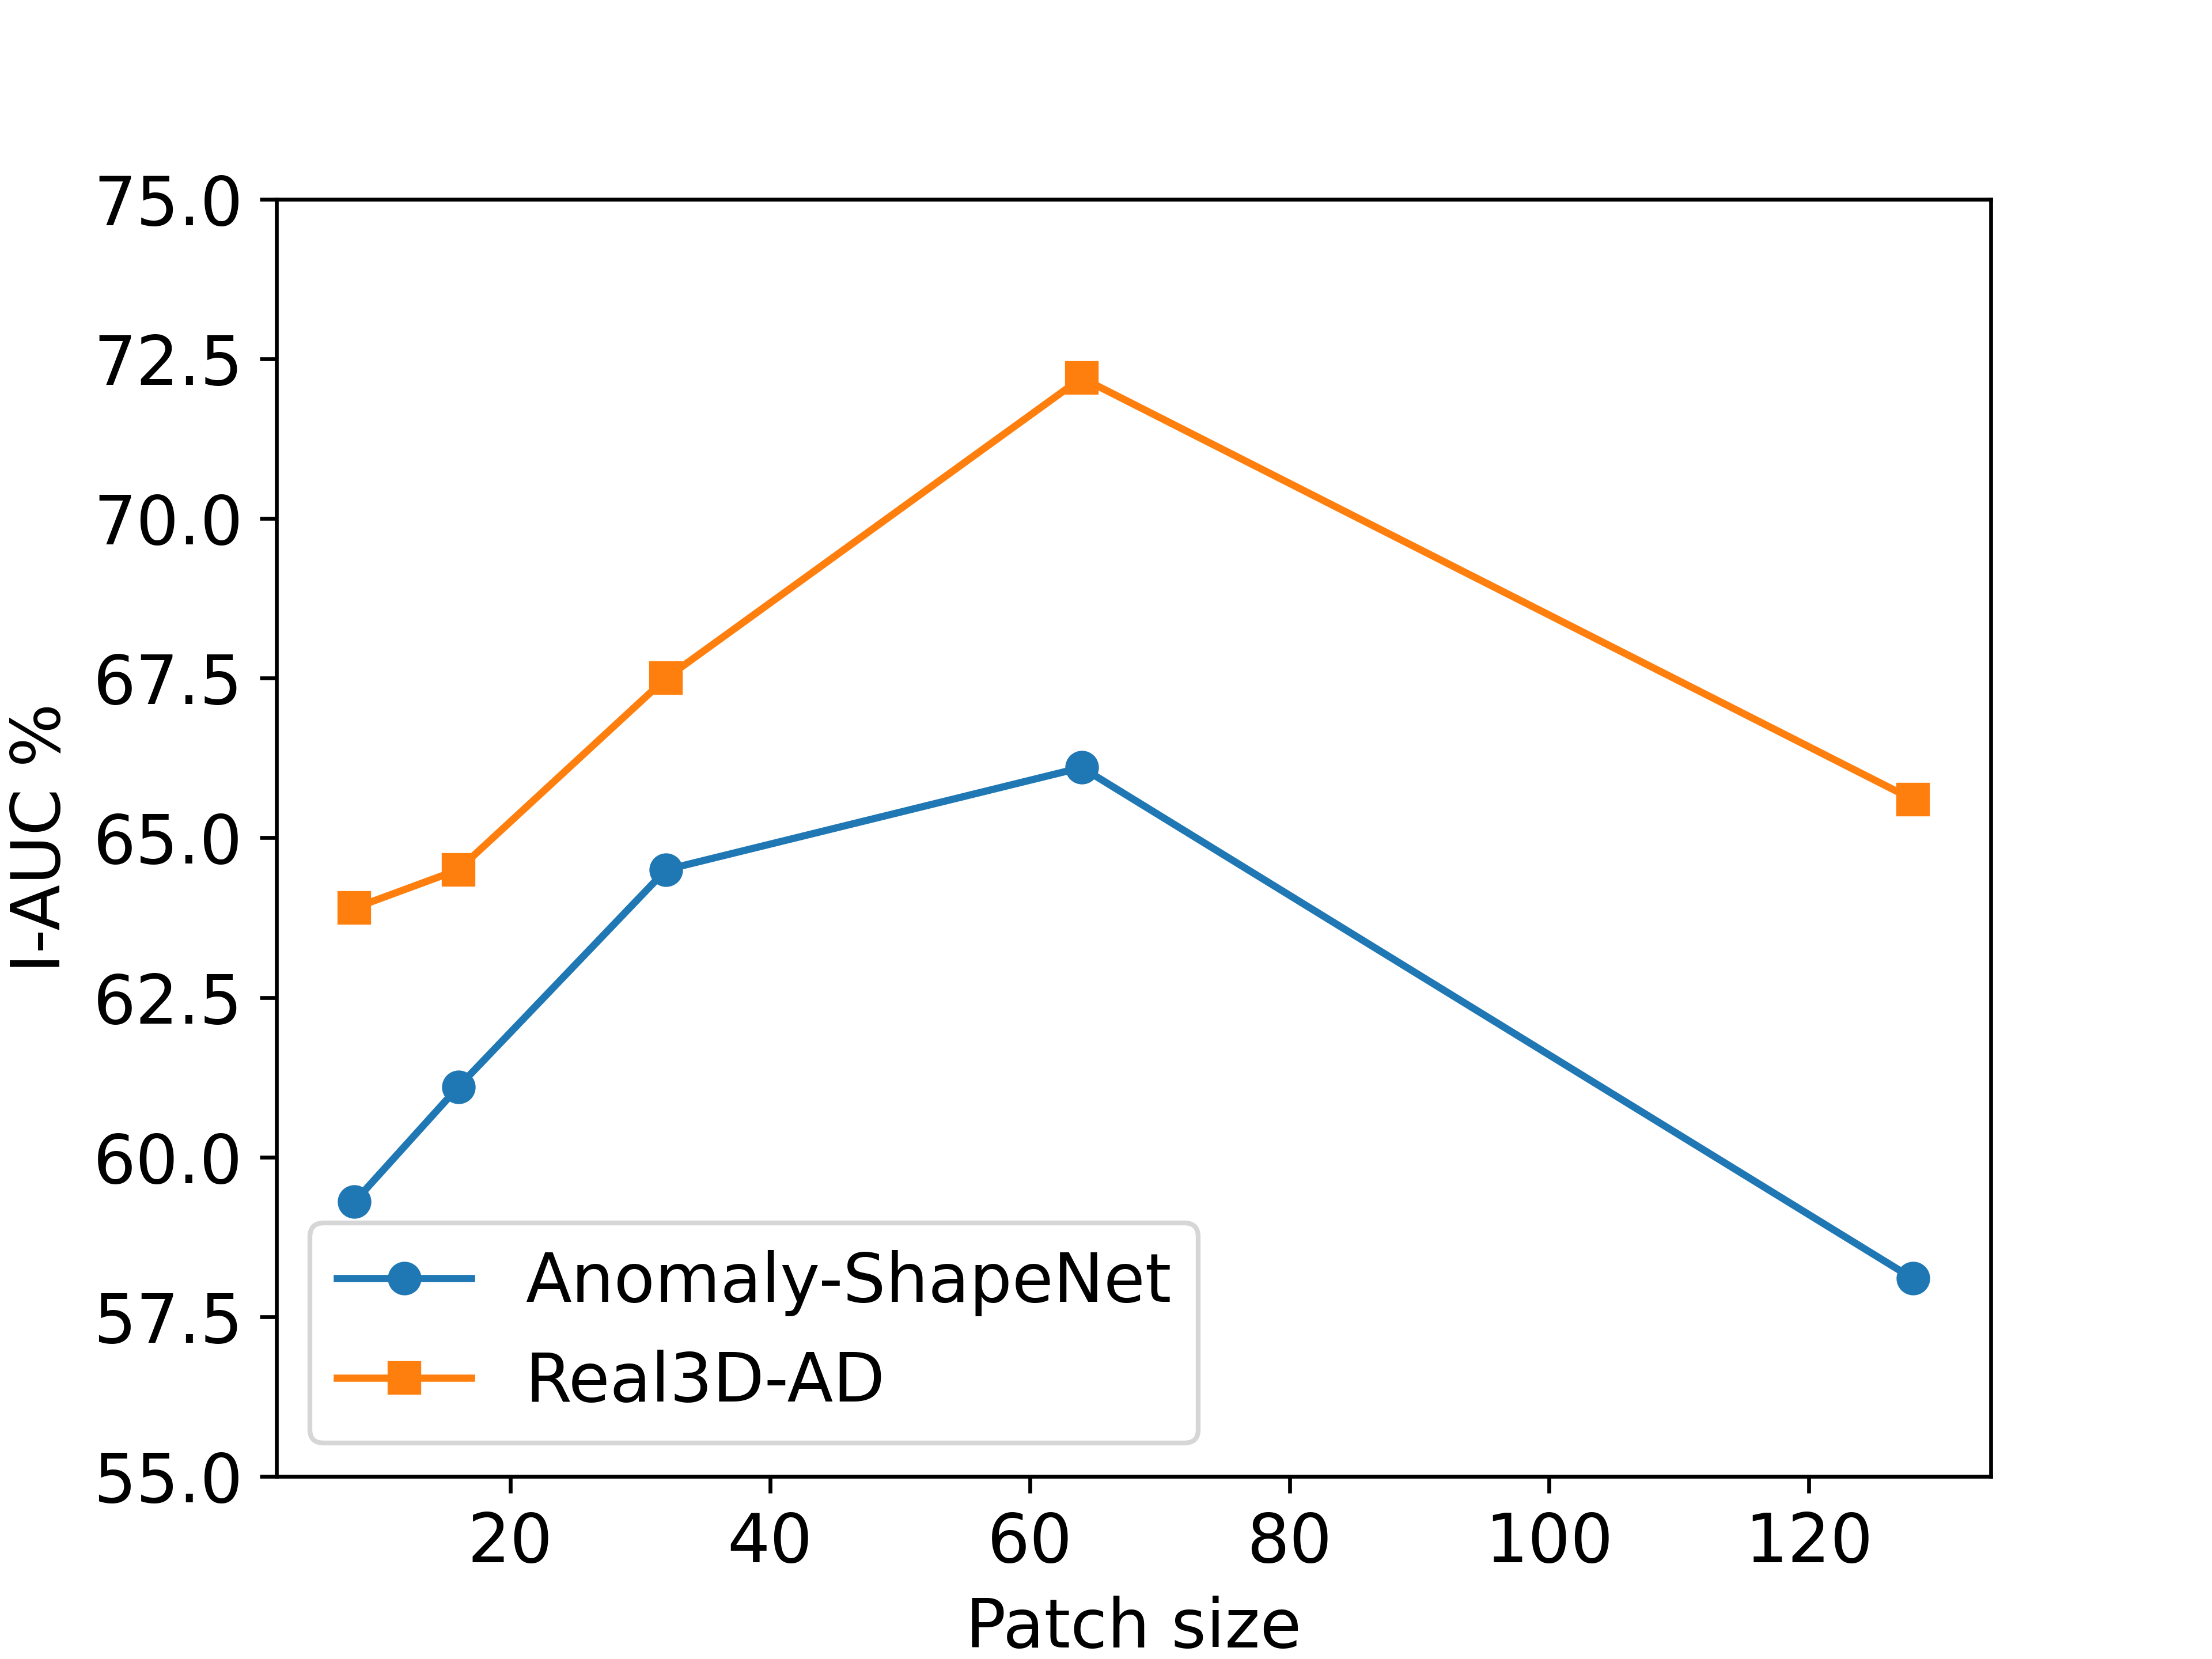}
            \label{fig:mask1}
        \end{minipage}
    }
    \vspace{-5pt}
     \caption{Ablation study of iteration number and patch size.}
      \vspace{-5pt}
     \label{fig:patch}
\label{fig:effect}
\end{figure*}
