# Supplementary material for: Towards Scalable 3D Anomaly Detection and Localization: A Benchmark via 3D Anomaly Synthesis and A Self-Supervised Learning Network
Source: arXiv:2311.14897 source file (2023-11-30)
Supplement: Supplementary file 2 [file vis.tex]

\begin{figure*}[htp]
\begin{center}
\vspace{-5mm}
\hspace{-5mm}
\subfloat{\includegraphics[width=\linewidth]{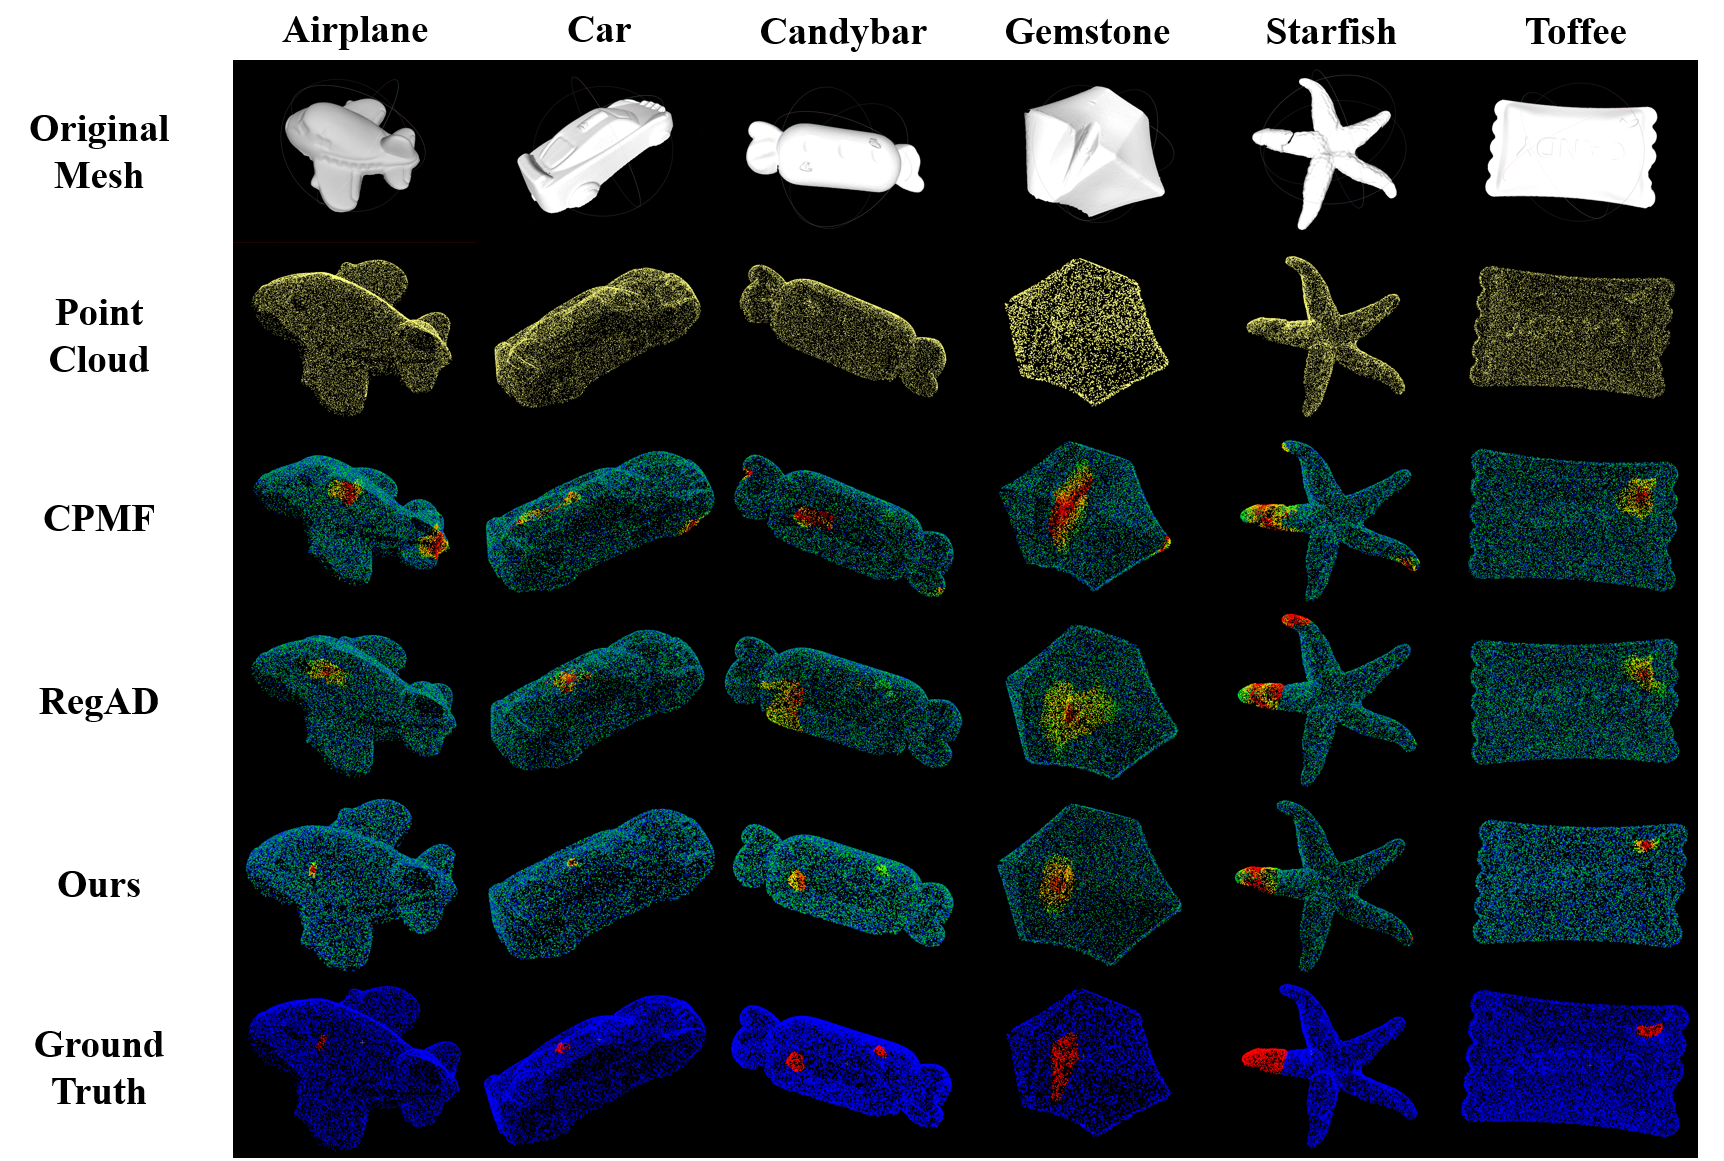}}\end{center}
\vspace{-2mm}
\caption{\textbf{Qualitative results visualization of anomaly localization performance on Real3D-AD.}}
\vspace{-2mm}
\label{fig:vis}
\end{figure*}
