# Supplementary material for: Towards Scalable 3D Anomaly Detection and Localization: A Benchmark via 3D Anomaly Synthesis and A Self-Supervised Learning Network
Source: arXiv:2311.14897 source file (2023-11-30)
Supplement: Supplementary file 3 [file 0_introduction.tex]

\setcounter{section}{0}
\setcounter{figure}{0}
\setcounter{table}{0}
\setcounter{equation}{0}

In this supplementary material, we provide 
more details that could not be included in the main manuscript due to the lack of space.
The contents are summarized below:

\begin{compactitem}[$\bullet$]
    \item \ref{sec:samples}. More Anomaly-ShapeNet anomaly samples.
    \item \ref{sec:visualization}.Visualization samples of Real3D-AD for anomaly detection and localization.
    \item \ref{sec:experiments}. Complete experiment results of IMRNet on anomaly detection and segmentation.
    \item \ref{sec:effect}. Ablation Study of iteration number and patch size. 
    \item \ref{sec:discussion}. Limitations and future works.
\end{compactitem}
