# Supplementary material for: Towards Scalable 3D Anomaly Detection and Localization: A Benchmark via 3D Anomaly Synthesis and A Self-Supervised Learning Network
Source: arXiv:2311.14897 source file (2023-11-30)
Supplement: Supplementary file 4 [file 1_samples.tex]

\section{Anomaly-ShapeNet Samples}
In this section, we present more anomalous examples of our proposed Anomaly-ShapeNet dataset. Figure \ref{s1} and \ref{s2} display the meshes and point clouds legends of six different anomaly types.
\label{sec:samples}
