# Supplementary material for: Towards Scalable 3D Anomaly Detection and Localization: A Benchmark via 3D Anomaly Synthesis and A Self-Supervised Learning Network
Source: arXiv:2311.14897 source file (2023-11-30)
Supplement: Supplementary file 5 [file 2_experiments.tex]

\section{Complete experiment results of IMRNet on anomaly detection and segmentation}
\label{sec:experiments}
To provide a comprehensive benchmark for our Anomaly-ShapeNet dataset, we tested different metrics on the Anomaly-ShapeNet dataset using mainstream 3D algorithms. The experimental results are presented in Table \ref{p-auc} and Table \ref{i-ap}
