# Supplementary material for: Towards Scalable 3D Anomaly Detection and Localization: A Benchmark via 3D Anomaly Synthesis and A Self-Supervised Learning Network
Source: arXiv:2311.14897 source file (2023-11-30)
Supplement: Supplementary file 6 [file 3_visualization.tex]

\section{Visualization samples of Real3D-AD for anomaly detection and localization.}
\label{sec:visualization}
Within the main text, we showcase a subset of the visualization results for anomaly detection and localization performed by the IMRNet algorithm on Anomaly-ShapeNet. Due to space constraints, the visualizations of IMRNet's detection results on Real-3D are presented in Figure \ref{fig:vis}. In this figure, the detection and localization performance of our IMRNet algorithm is evidently superior to that of the CPMF and RegAD algorithms.
