# Supplementary material for: Towards Scalable 3D Anomaly Detection and Localization: A Benchmark via 3D Anomaly Synthesis and A Self-Supervised Learning Network
Source: arXiv:2311.14897 source file (2023-11-30)
Supplement: Supplementary file 7 [file 4_effect.tex]

\section{Ablation study of iteration number and patch size.}
In the main text, we present the experimental results demonstrating the correlation between the effectiveness of IMRNet's anomaly detection and the masking rate. As a supplement, we provide the relationship curves between anomaly detection performance, mask size, and iteration number in Figure \ref{fig:effect} to aid in understanding the relation of experimental parameters and the detection effect. Figure \ref{fig:effect} demonstrate the best iteration time and patch size are 3 and 64. Theoretically, larger iteration time and patch size may induce normal point drift and increase the positive false rate, while smaller ones may be not enough to cover all anomaly regions. 
\label{sec:effect}
