# Supplementary material for: Towards Scalable 3D Anomaly Detection and Localization: A Benchmark via 3D Anomaly Synthesis and A Self-Supervised Learning Network
Source: arXiv:2311.14897 source file (2023-11-30)
Supplement: Supplementary file 8 [file 5_discussion.tex]

\section{Limitations and future works.}
\label{sec:discussion}

Our proposed Anomaly-ShapeNet dataset, while encompassing a broad distribution of samples, still lacks sufficient scale. Future work will need to focus on expanding the number of samples within the dataset. Moreover, Pure point cloud coordinate-based 3D anomaly detection does not fully conform to real-world 3D anomaly detection scenarios. Subsequent efforts should involve the integration of RGB values into our anomaly detection model.
\begin{figure*}[htp]
\begin{center}
\vspace{-5mm}
\hspace{-5mm}
\subfloat{\includegraphics[width=\linewidth]{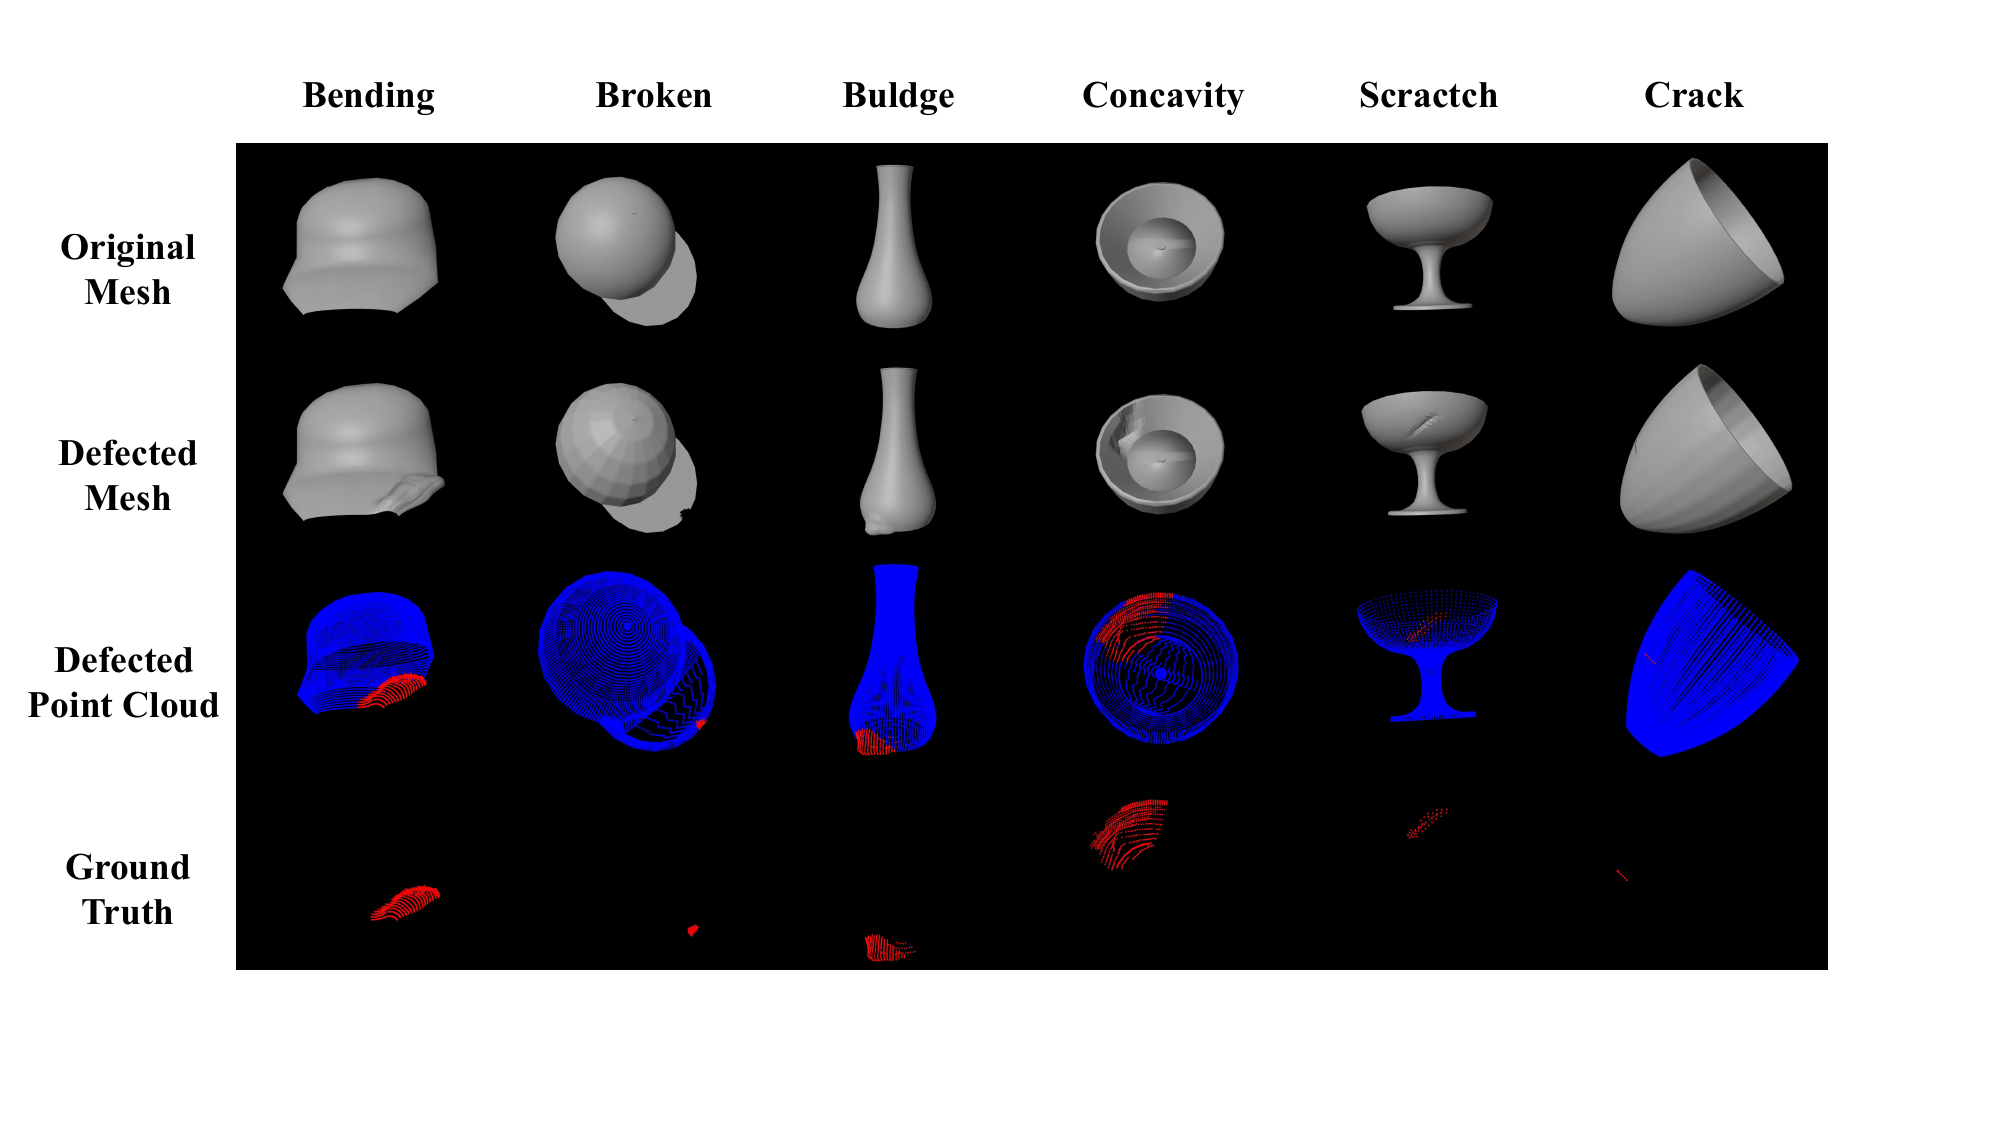}}\end{center}
\vspace{-7mm}
\caption{\textbf{Examples of the proposed Anomaly-ShapeNet}}
\vspace{-2mm}
\label{s1}
\end{figure*}
\begin{figure*}[htp]
\begin{center}
\vspace{-5mm}
\hspace{-5mm}
\subfloat{\includegraphics[width=\linewidth]{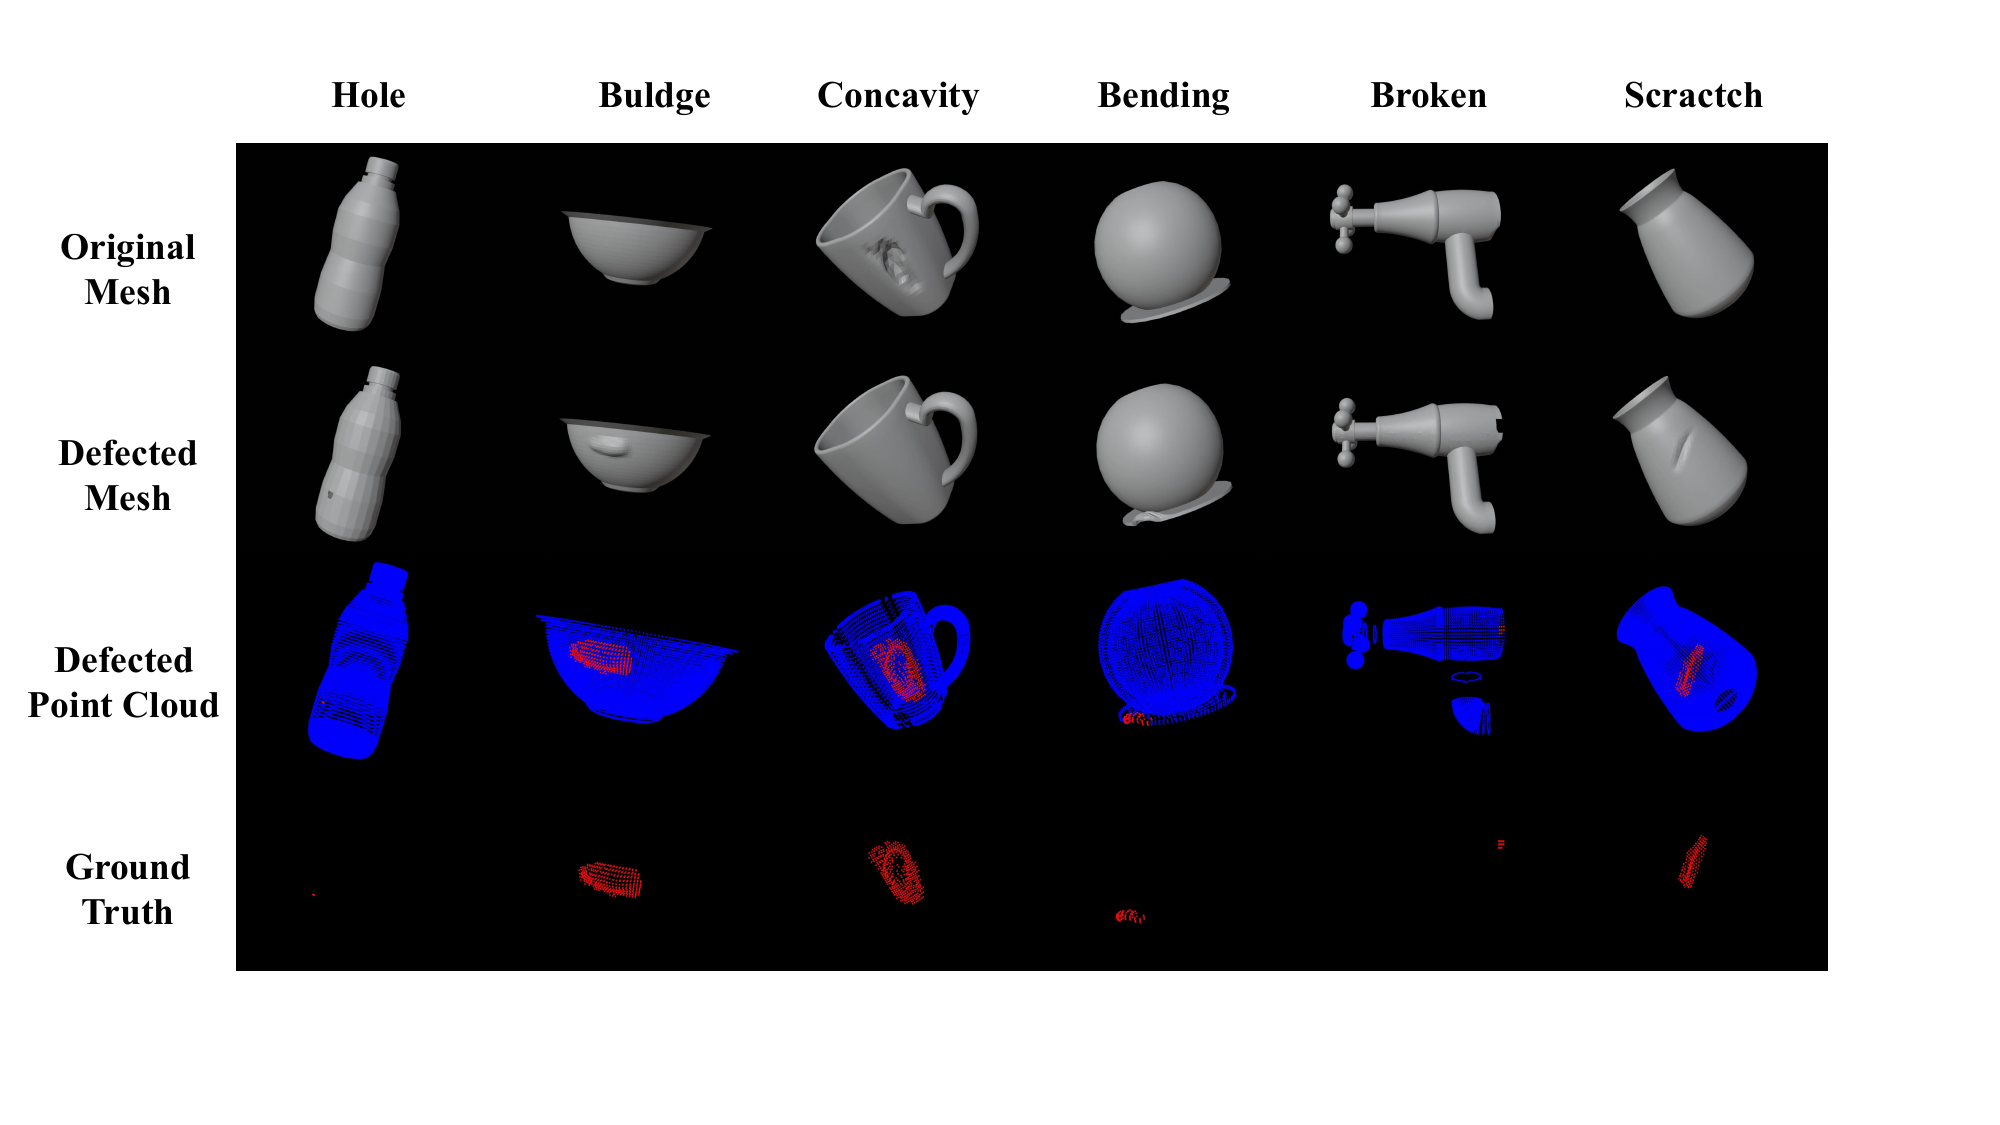}}\end{center}
\vspace{-7mm}
\caption{\textbf{Examples of the proposed Anomaly-ShapeNet.}}
\vspace{-2mm}
\label{s2}
\end{figure*}
\begin{figure*}[htp]
\begin{center}
\vspace{-5mm}
\hspace{-5mm}
\subfloat{\includegraphics[width=\linewidth]{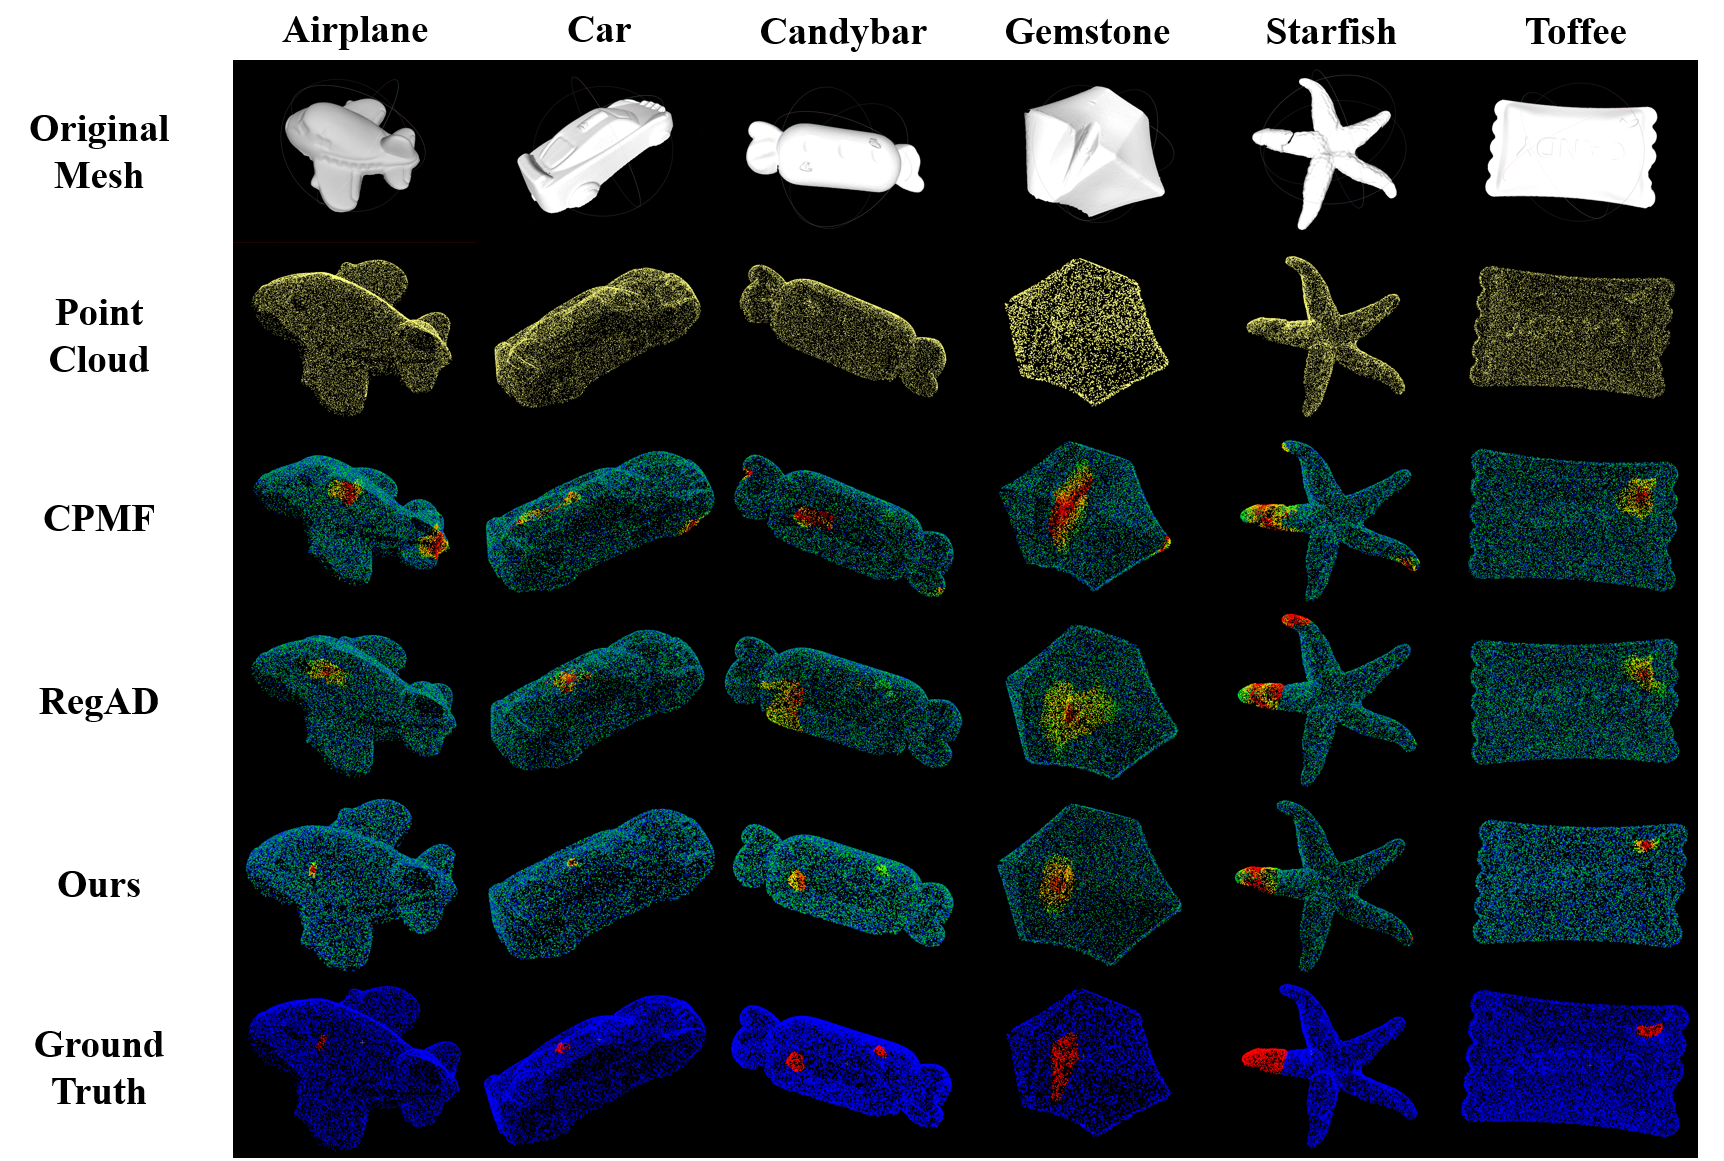}}\end{center}
\vspace{-2mm}
\caption{\textbf{Qualitative results visualization of anomaly localization performance on Real3D-AD.}}
\vspace{-2mm}
\label{fig:vis}
\end{figure*}
% \vspace{-4mm}

% \end{figure}
\begin{figure*}
    \subfloat[Iteration number influence.]{
        \begin{minipage}[t]{0.46\linewidth}
            \centering
            \includegraphics[width=0.9\linewidth]{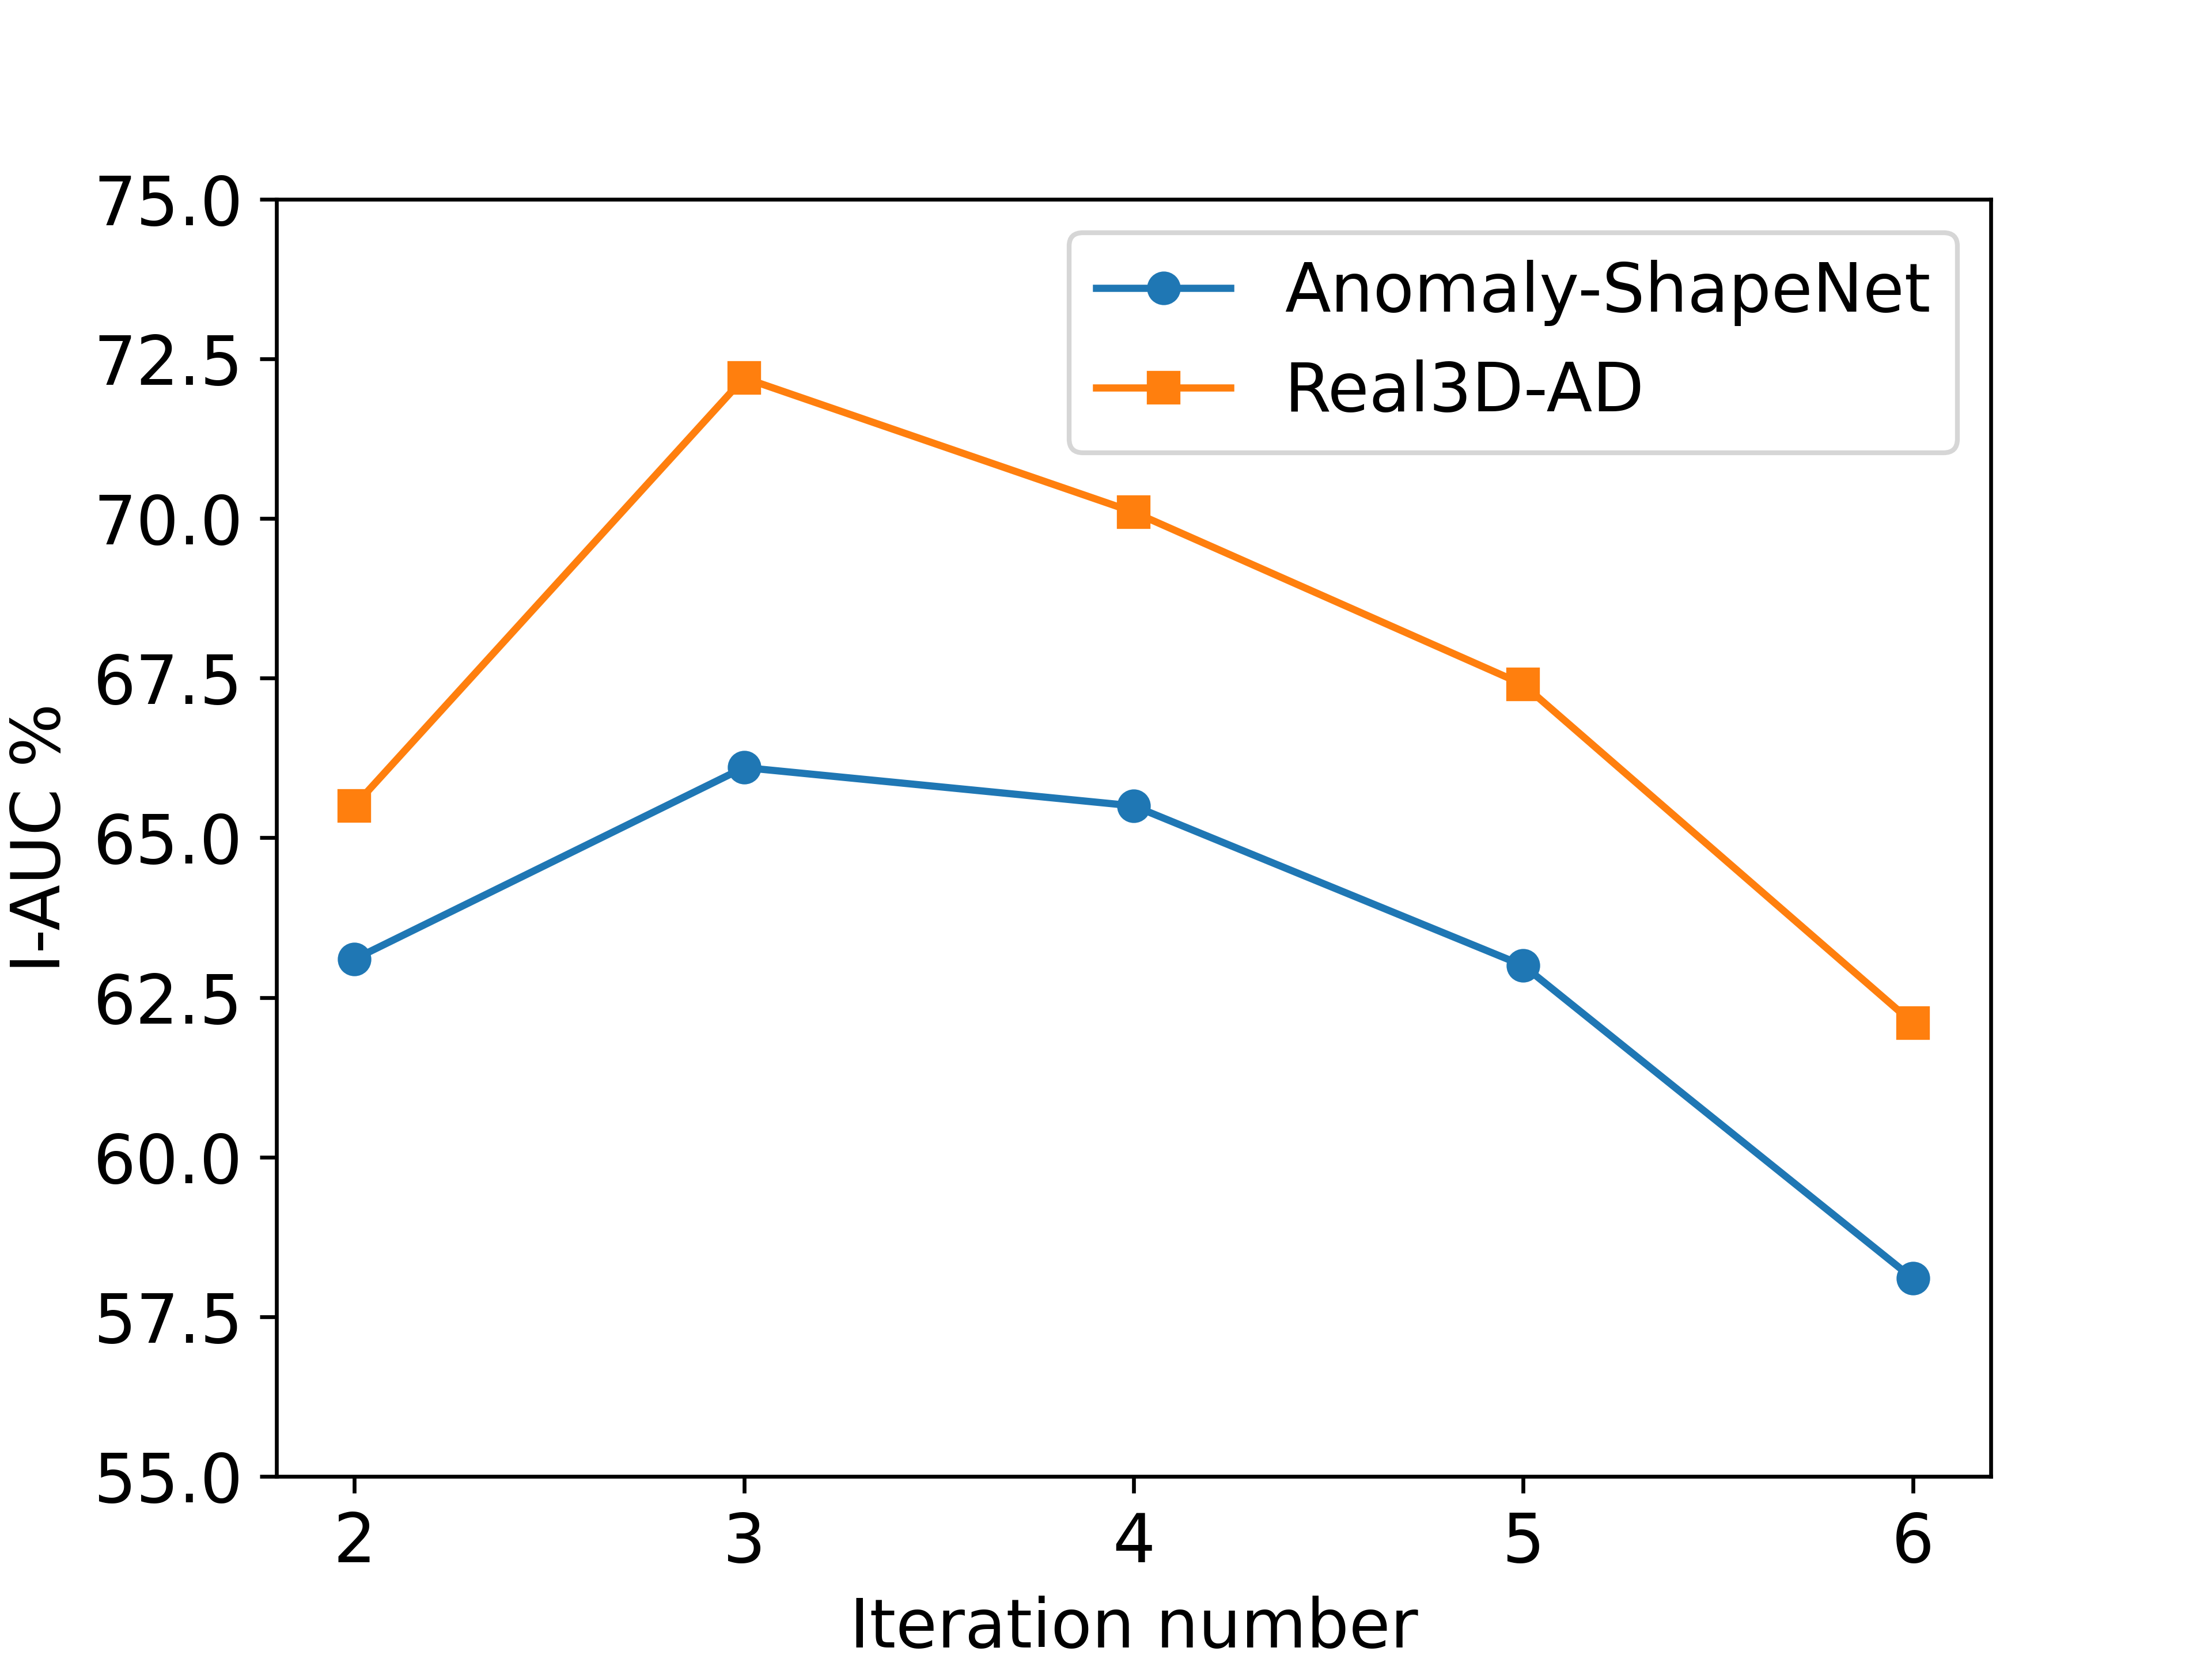}
            \label{fig:iter}
        \end{minipage}
    }
    \hfill
    \subfloat[Patch size influence.]{
        \begin{minipage}[t]{0.46\linewidth}
            \centering
            \includegraphics[width=0.9\linewidth]{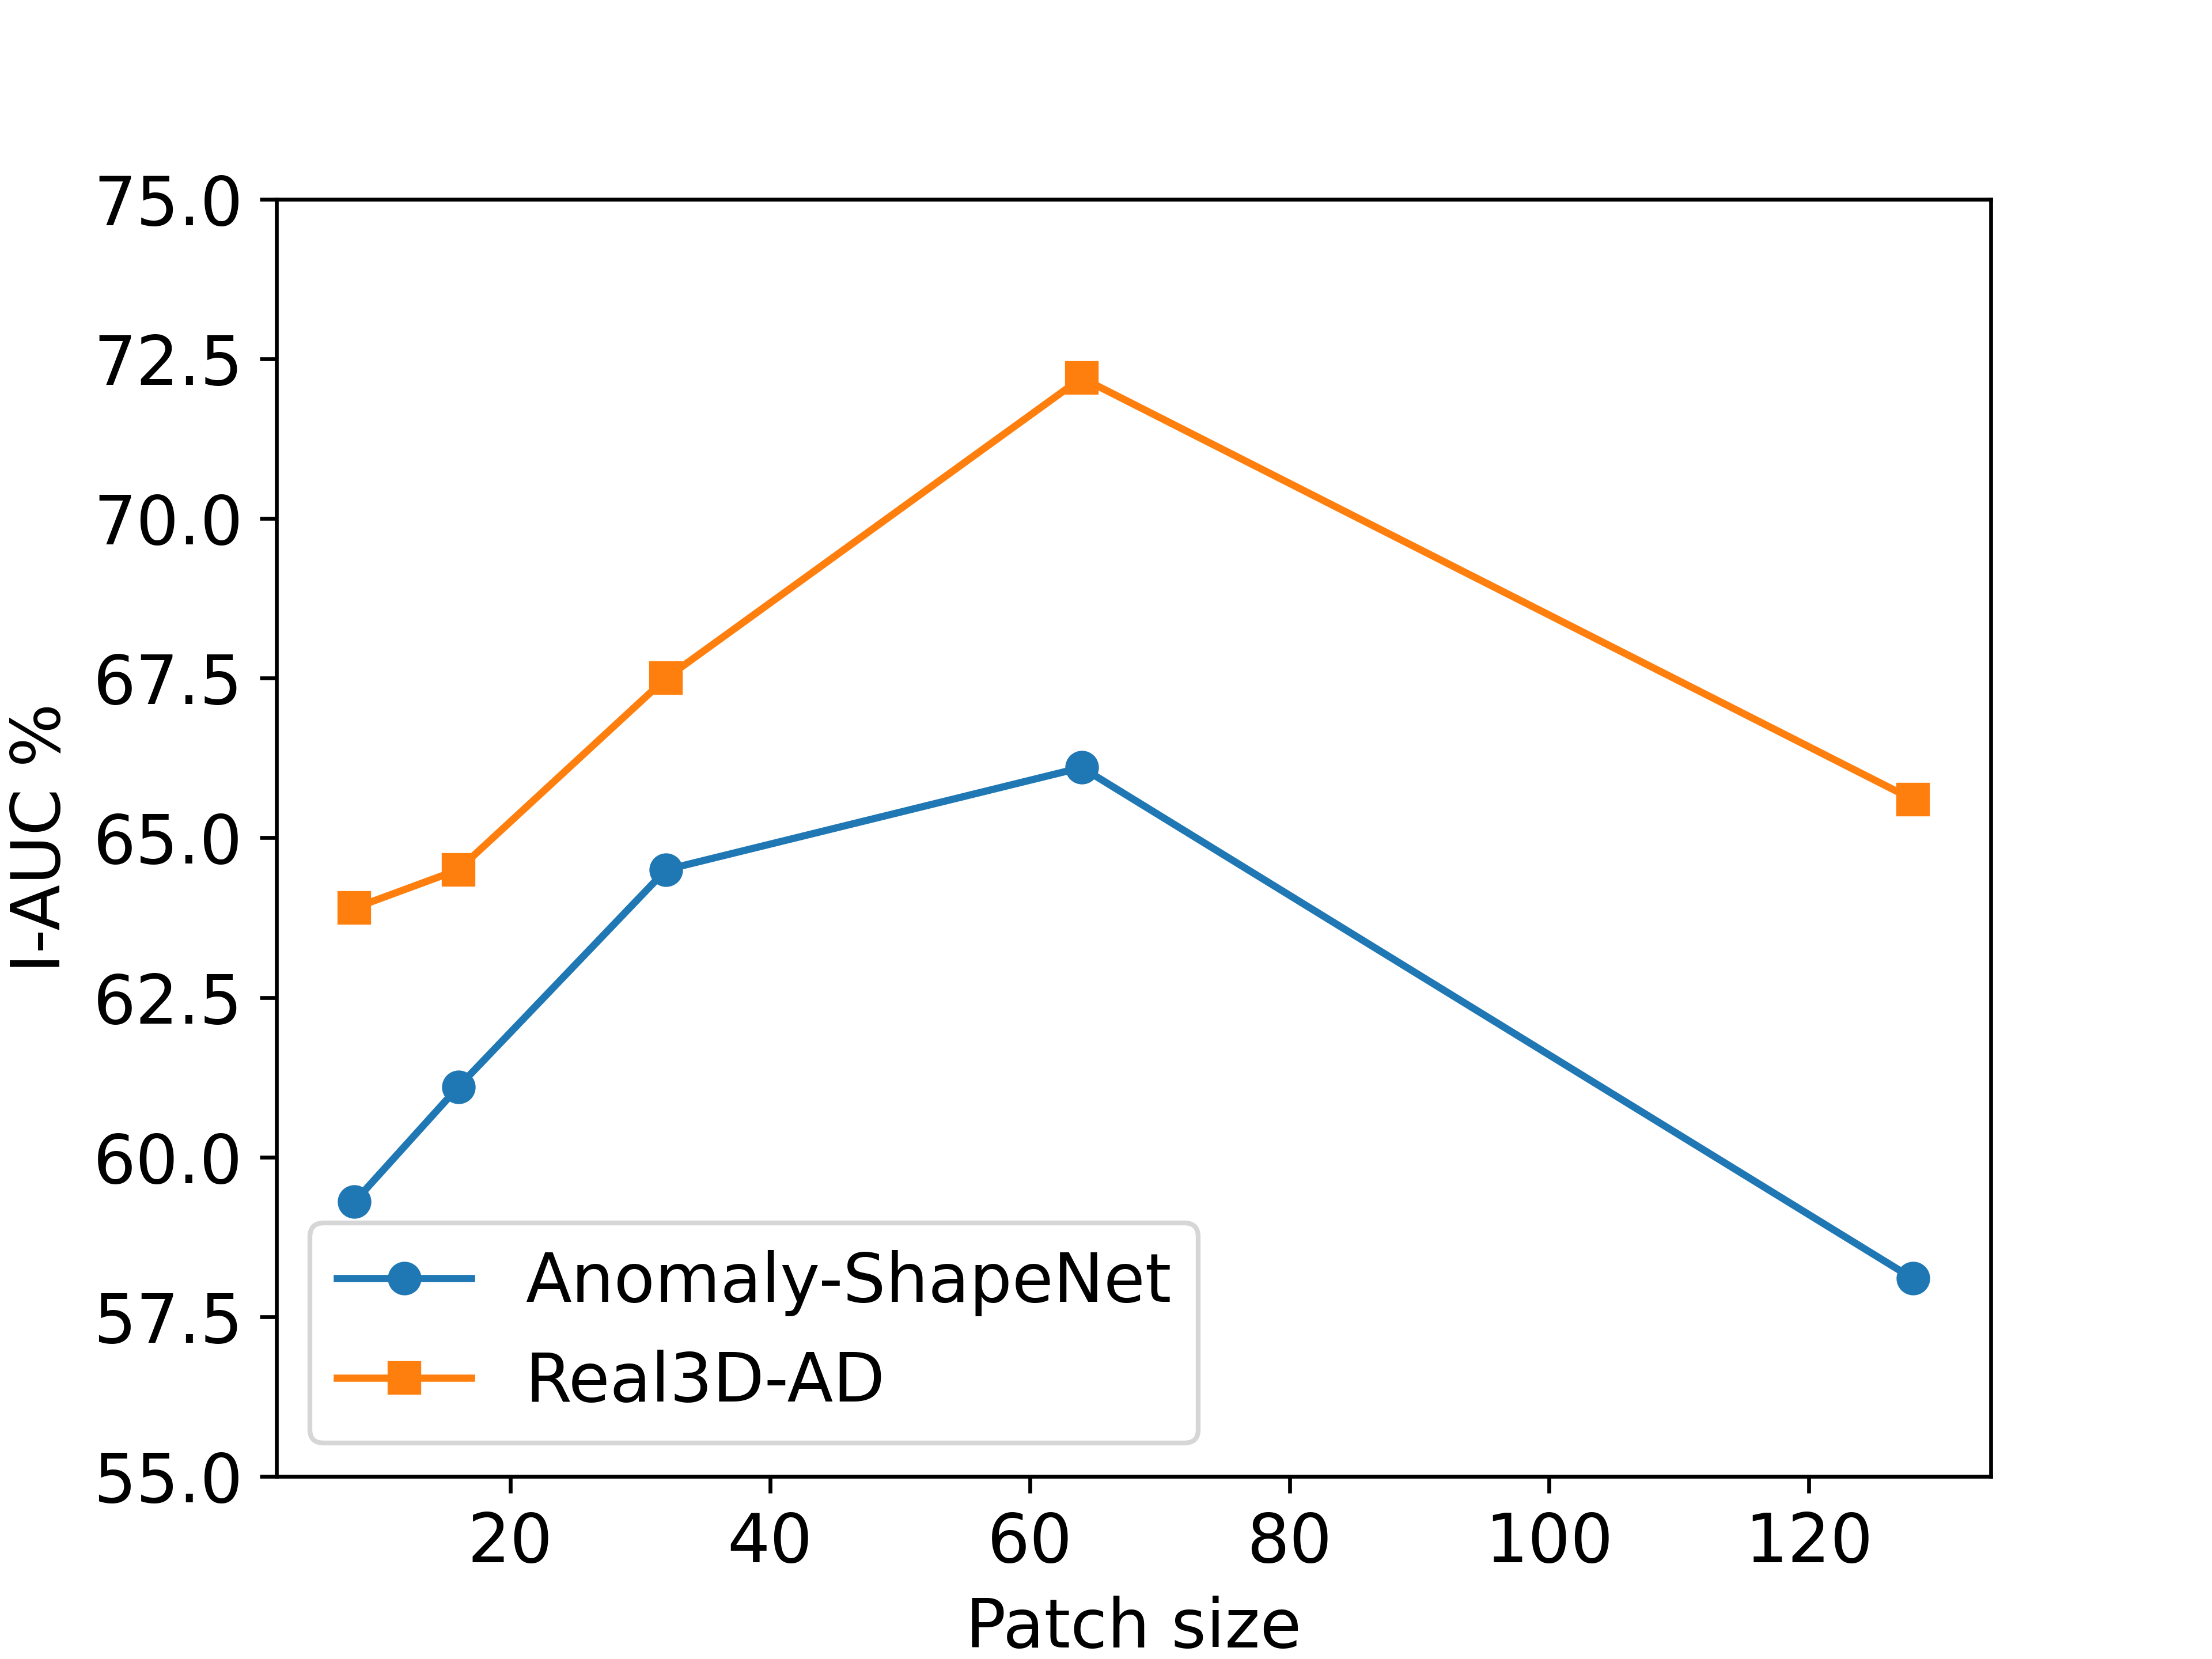}
            \label{fig:mask1}
        \end{minipage}
    }
    \vspace{-5pt}
     \caption{Ablation study of iteration number and patch size.}
      \vspace{-5pt}
     \label{fig:patch}
\label{fig:effect}
\end{figure*}
\begin{table*}
  \vspace{-10pt}
  \centering
  \scriptsize
  
  \begin{tabular}{@{}cl|m{0.6cm}<{\centering}m{0.6cm}<{\centering}m{0.6cm}<{\centering}m{0.6cm}<{\centering}m{0.6cm}<{\centering}m{0.6cm}<{\centering}m{0.6cm}<{\centering}m{0.65cm}<{\centering}m{0.65cm}<{\centering}m{0.6cm}<{\centering}m{0.6cm}<{\centering}m{0.6cm}<{\centering}m{0.6cm}<{\centering} m{0.6cm}<{\centering}}
    \toprule
    & Method & cap0 & cap3 &helmet3  & cup0 & bowl4 & vase3 & headset1 & eraser0 & vase8 & cap4 &vase2 & vase4 & helmet0 & bucket1\\
    \midrule 
     &BTF(Raw) & 0.524 & 0.687 & 0.700 & 0.632 & 0.563 & 0.602 & 0.475 & 0.637 & 0.550 & 0.469 & 0.403&0.613 &0.504&0.686 \\
     &BTF(FPFH) & 0.730 & 0.658 & 0.724 & 0.790 & 0.679 & 0.699 & 0.591 & 0.719 & 0.662 & 0.524 & 0.646 &0.710 &0.575&0.633 \\
     &M3DM & 0.531 & 0.605 & 0.655 & 0.715 & 0.624 & 0.658 & 0.585 & 0.710 & 0.551 & 0.718 & 0.737&0.655 &0.599&0.699 \\
     &Patchcore(FPFH) & 0.472 & 0.653 & 0.737& 0.655 & 0.720 & 0.430 & 0.464 & 0.810 & 0.575 & 0.595 & 0.721&0.505 &0.548&0.571 \\
     &Patchcore(PointMAE) & 0.544  & 0.488 & 0.615 & 0.510 & 0.501 & 0.465 & 0.423 & 0.378 & 0.364 &0.725 & 0.742&0.523 &0.580&0.574 \\
     &CPMF & 0.601 & 0.551 & 0.520 & 0.497 & 0.683 & 0.582 & 0.458 & 0.689 & 0.529 & 0.553 & 0.582&0.514 &0.555&0.601\\
     &RegAD & 0.632 & 0.718 & 0.620 &0.685& 0.800 & 0.511 & 0.626 & 0.755 & 0.811 & 0.815 & 0.405 & 0.755&0.600 &0.752\\
     &\textbf{Ours} &  0.715 & 0.706 &  0.663 &  0.643 & 0.576 & 0.401  & 0.476 & 0.548 &0.635 & 0.753 &0.614 &0.524 & 0.598&0.774\\
     \midrule
    \midrule
    & Method & bottle3 & vase0 & bottle0 & tap1 & bowl0 & bucket0 & vase5 & vase1 & vase9 & ashtray0 & bottle1 & tap0 & phone & cup1\\
    \midrule 
     &BTF(Raw) & 0.720 & 0.618 & 0.551 & 0.564 & 0.524 & 0.617 & 0.585 & 0.549 & 0.564 & 0.512 & 0.491&0.527 &0.583&0.561 \\
     &BTF(FPFH) & 0.622 & 0.642 & 0.641 & 0.596 & 0.710 & 0.401 & 0.429 & 0.619 & 0.568 & 0.624 & 0.549 &0.568 &0.675&0.619 \\
     &M3DM & 0.532 & 0.608 & 0.663 & 0.712 & 0.658 & 0.698 & 0.642 & 0.602 & 0.663 & 0.577 & 0.637&0.654 &0.358&0.556 \\
     &Patchcore(FPFH) & 0.512 & 0.655 & 0.654& 0.768 & 0.524 & 0.459 & 0.447 & 0.453 & 0.663 & 0.597 & 0.687&0.733 &0.488&0.596 \\
     &Patchcore(PointMAE) & 0.653  & 0.677 & 0.553 & 0.541 & 0.527 & 0.586 & 0.572 & 0.551 & 0.423 &0.495 & 0.606&0.858 &0.886&0.856 \\
     &CPMF & 0.435 & 0.458 & 0.521 & 0.657 & 0.745 & 0.486 & 0.651 & 0.486 & 0.545 & 0.615 & 0.571&0.458 &0.545&0.509\\
     &RegAD & 0.525 & 0.548 & 0.886 & 0.741 & 0.775 & 0.619 & 0.624 & 0.602 & 0.694 & 0.698 & 0.696&0.589 &0.599&0.698\\
     &\textbf{Ours} & 0.641 & 0.535 &  0.556 & 0.699 &  0.781 & 0.585 & 0.682 & 0.685&0.691&0.671&0.702 & 0.681&0.742&0.688 \\
    \midrule
    \midrule
    & Method & vase7 & helmet2  & cap5 & shelf0 & bowl5 & bowl3 & helmet1 & bowl1 & headset0 & bag0& bowl2 & jar& \multicolumn{2}{|c}{\textbf{Mean}} \\
    \midrule 
     &BTF(Raw) & 0.578 & 0.605  & 0.373 & 0.464 & 0.517 & 0.685 & 0.449 & 0.464 & 0.578 & 0.430&0.426 &0.423&\multicolumn{2}{|c}{0.550} \\
     &BTF(FPFH) & 0.540 & 0.643  & 0.586 & 0.619 & 0.699 & 0.590 & 0.749 & 0.768 & 0.620 & 0.746 &0.518 &0.427&\multicolumn{2}{|c}{0.628} \\
     &M3DM & 0.517 & 0.623  & 0.655 & 0.554 & 0.489 & 0.657 & 0.427 & 0.663 & 0.581 & 0.637&0.694 &0.541&\multicolumn{2}{|c}{0.616} \\
     &Patchcore(FPFH) & 0.693 & 0.455 &  0.795 & 0.613 & 0.358 & 0.327 & 0.489 & 0.531 & 0.583 & 0.574&0.625 &0.478&\multicolumn{2}{|c}{0.580} \\
     &Patchcore(PointMAE) & 0.651  & 0.651  & 0.545 & 0.543 & 0.562 & 0.581 & 0.562 & 0.524 &0.575 & 0.674&0.515 &0.487&\multicolumn{2}{|c}{0.577} \\
     &CPMF & 0.504 & 0.515  & 0.551 & 0.783 & 0.684 & 0.641 & 0.542 & 0.488 & 0.699 & 0.655&0.635&0.611&\multicolumn{2}{|c}{0.573}\\
     &RegAD & 0.881& 0.825  & 0.467 &0.688 & 0.691 & 0.654 & 0.624 & 0.615 & 0.580 & 0.715&0.593 &0.599&\multicolumn{2}{|c}{0.668}\\
     &\textbf{Ours} & 0.593 & 0.644  & 0.742 &  0.605 &0.715 & 0.599 & 0.604& 0.705 &  0.705 &0.668 &0.684 &0.765 & \multicolumn{2}{|c}{0.650}\\
    \bottomrule
  \end{tabular}
  \vspace{5pt}
  \caption{\textbf{P-AUROC score for anomaly detection of 40 categories of our Anomaly-ShapeNet dataset}}
  \vspace{-10pt}
  \label{p-auc}
\end{table*}
\begin{table*}
  \vspace{-10pt}
  \centering
  \scriptsize
  
  \begin{tabular}{@{}cl|m{0.6cm}<{\centering}m{0.6cm}<{\centering}m{0.6cm}<{\centering}m{0.6cm}<{\centering}m{0.6cm}<{\centering}m{0.6cm}<{\centering}m{0.6cm}<{\centering}m{0.65cm}<{\centering}m{0.65cm}<{\centering}m{0.6cm}<{\centering}m{0.6cm}<{\centering}m{0.6cm}<{\centering}m{0.6cm}<{\centering} m{0.6cm}<{\centering}}
    \toprule
    & Method & cap0 & cap3 &helmet3  & cup0 & bowl4 & vase3 & headset1 & eraser0 & vase8 & cap4 &vase2 & vase4 & helmet0 & bucket1\\
    \midrule 
     &BTF(Raw) & 0.659 & 0.612 & 0.526 & 0.601 & 0.601 & 0.717 & 0.515 & 0.425 & 0.416 & 0.515 & 0.413&0.428 &0.559&0.620 \\
     &BTF(FPFH) & 0.618 & 0.579 & 0.564 & 0.585 & 0.632 & 0.652 & 0.523 & 0.719 & 0.624 & 0.545 & 0.569 &0.587 &0.568&0.648 \\
     &M3DM & 0.564 & 0.652 & 0.458 & 0.570 & 0.571 & 0.551 & 0.623 & 0.625 & 0.463 & 0.477 & 0.615&0.526 &0.528&0.507 \\
     &Patchcore(FPFH) & 0.585 & 0.457 & 0.494& 0.604 & 0.575 & 0.481 & 0.601 & 0.584 & 0.515 & 0.655 & 0.801&0.777 &0.525&0.565 \\
     &Patchcore(PointMAE) & 0.561  & 0.583 & 0.611 & 0.642 & 0.601 & 0.455 & 0.423 & 0.801 & 0.655 &0.721 & 0.711&0.586 &0.633&0.642 \\
     &CPMF & 0.601 & 0.541 & 0.645 & 0.647 & 0.683 & 0.588 & 0.619 & 0.544 & 0.673 & 0.645 & 0.632&0.655 &0.333&0.501\\
     &RegAD & 0.693 & 0.711 & 0.468 &0.531& 0.624 & 0.651 & 0.617 & 0.424 & 0.629 & 0.623 & 0.641 & 0.505&0.600 &0.714\\
     &\textbf{Ours} &  0.711 & 0.702 &  0.575 &  0.455 & 0.630 & 0.708  & 0.656 & 0.599 &0.639 & 0.658 &0.655 &0.528 & 0.697&0.732\\
     \midrule
    \midrule
    & Method & bottle3 & vase0 & bottle0 & tap1 & bowl0 & bucket0 & vase5 & vase1 & vase9 & ashtray0 & bottle1 & tap0 & phone & cup1\\
    \midrule 
     &BTF(Raw) & 0.543 & 0.562 & 0.466 & 0.594 & 0.588 & 0.652 & 0.615 & 0.441 & 0.482 & 0.578 & 0.573&0.535 &0.613&0.701 \\
     &BTF(FPFH) & 0.602 & 0.641 & 0.644 & 0.575 & 0.576 & 0.483 & 0.472 & 0.655 & 0.638 & 0.651 & 0.625 &0.610 &0.662&0.651 \\
     &M3DM & 0.451 & 0.788 & 0.763 & 0.638 & 0.525 & 0.609 & 0.633 & 0.652 & 0.651 & 0.632 & 0.674&0.722 &0.464&0.752 \\
     &Patchcore(FPFH) & 0.579 & 0.645 & 0.615&0.684 & 0.548 & 0.604 & 0.515 & 0.623 & 0.660 & 0.445 & 0.677&0.712 &0.332&0.586 \\
     &Patchcore(PointMAE) & 0.651  & 0.548 & 0.545& 0.542 & 0.562 & 0.541 & 0.585 & 0.572 & 0.634 &0.679 & 0.645&0.712 &0.652&0.710 \\
     &CPMF & 0.505 & 0.632 & 0.588 & 0.697 & 0.775 & 0.662 & 0.518 & 0.645 & 0.618 & 0.453 & 0.592&0.639 &0.655&0.609\\
     &RegAD & 0.474 & 0.615 & 0.632 & 0.599 & 0.494 & 0.632 & 0.588 & 0.468 & 0.574 & 0.588 & 0.695&0.676 &0.614&0.638\\
     &\textbf{Ours} & 0.648 & 0.573 &  0.558 & 0.796 &  0.481 & 0.578 & 0.654 & 0.725&0.462&0.612&0.702 & 0.401&0.552 &0.627 \\
    \midrule
    \midrule
    & Method & vase7 & helmet2  & cap5 & shelf0 & bowl5 & bowl3 & helmet1 & bowl1 & headset0 & bag0& bowl2 & jar& \multicolumn{2}{|c}{\textbf{Mean}} \\
    \midrule 
     &BTF(Raw) & 0.547 & 0.615  & 0.653 & 0.624 & 0.615 & 0.654 & 0.388 & 0.464 & 0.379 & 0.458&0.576 &0.428&\multicolumn{2}{|c}{0.549} \\
     &BTF(FPFH) & 0.592 & 0.588  & 0.593 & 0.611 & 0.699 & 0.499 & 0.721 & 0.648 & 0.531 & 0.551 &0.515 &0.479&\multicolumn{2}{|c}{0.598} \\
     &M3DM & 0.648 & 0.636  & 0.642 & 0.665 & 0.601 & 0.635 & 0.627 & 0.515 & 0.632 & 0.642&0.630 &0.555&\multicolumn{2}{|c}{0.603} \\
     &Patchcore(FPFH) & 0.621 & 0.475 & 0.725 & 0.504 & 0.541 & 0.620 & 0.630 & 0.545 & 0.701 & 0.608&0.611 &0.499&\multicolumn{2}{|c}{0.588} \\
     &Patchcore(PointMAE) & 0.652  & 0.496  & 0.542 & 0.543 & 0.585 & 0.556 & 0.571 & 0.611 &0.515 & 0.601&0.456 &0.463&\multicolumn{2}{|c}{0.595} \\
     &CPMF & 0.432 & 0.477  & 0.697 & 0.681 & 0.685 & 0.418 & 0.501 & 0.621 & 0.602 & 0.655&0.601 &0.618&\multicolumn{2}{|c}{0.597}\\
     &RegAD & 0.455& 0.618  & 0.77 &0.675 & 0.555 & 0.441 & 0.381 & 0.515 & 0.538 & 0.608&0.495 &0.601&\multicolumn{2}{|c}{0.584}\\
     &\textbf{Ours} & 0.601 & 0.602 & 0.502 &  0.625 & 0.652 & 0.614 & 0.615& 0.504 & 0.701 &0.665 &0.681 &0.760 & \multicolumn{2}{|c}{0.621}\\
    \bottomrule
  \end{tabular}
  \vspace{-5pt}
  \caption{\textbf{I-AP score for anomaly detection of 40 categories of our Anomaly-ShapeNet dataset}}
  \vspace{-10pt}
  \label{i-ap}
\end{table*}
