# Supplementary material for: Towards Scalable 3D Anomaly Detection and Localization: A Benchmark via 3D Anomaly Synthesis and A Self-Supervised Learning Network
Source: arXiv:2311.14897 source file (2023-11-30)
Supplement: Supplementary file 9 [file 6_license.tex]

\subsection*{License of the used assets}

\begin{compactitem}[$\bullet$]
    \item InterHand2.6M dataset~\cite{moon2020interhand2} is CC-BY-NC 4.0 licensed.
    \item YT-3D dataset~\cite{kulon2020weakly} is Ariel AI licensed.
    \item \href{https://github.com/microsoft/MeshTransformer}{METRO~\cite{lin2021end} codes} are released for academic research only and it is free to researchers from educational or research institutes for non-commercial purposes. % code example
    \item \href{https://github.com/mks0601/Hand4Whole_RELEASE}{Pose2Pose~\cite{moon2022accurate} codes} are released for academic research only and it is free to researchers from educational or research institutes for non-commercial purposes. % code example
    \item \href{https://github.com/mks0601/I2L-MeshNet_RELEASE}{I2L-MeshNet~\cite{moon2020i2l} codes} are released for academic research only and it is free to researchers from educational or research institutes for non-commercial purposes. % code example

\end{compactitem}

\input{latex/supple/figures/YT3D_comparison_first}
\input{latex/supple/figures/BlurHand_comparison.tex}
