# Supplementary material for: Towards Scalable 3D Anomaly Detection and Localization: A Benchmark via 3D Anomaly Synthesis and A Self-Supervised Learning Network
Source: arXiv:2311.14897 source file (2023-11-30)
Supplement: Supplementary file 10 [file 7_comparison_under_same_cost.tex]

\section{Number of unfolding under the same cost}
% \label
In Table~\ref{reb_tab:efficiency}, we report the performance of BlurHandNet with different numbers of unfolding steps.
Since the 
For a fair comparison, we keep the number of parameters the same by adjusting the channel size.
The results demonstrate that the performance improvement is not due to a larger network capacity.
\begin{table}[!t]
    \vspace{-3mm}
    \centering
    \resizebox{0.8\linewidth}{!}{
    \begin{tabular}{l|ccc}
        \toprule
        \;~\# of unfolding & 1 & 3~(Ours) & 5\\
        \midrule
        % \,~GMACs~(\jaeha{unit}) & 13.59 & 30.02 & 46.44\\
        % \,~$\#$ of params~(M) &  & 85.36 & 85.39 \\
        \,~MPJPE (middle) & 17.48 & \textbf{16.80} & 16.91\\
        \bottomrule
    \end{tabular}
    }
    \vspace{-3mm}
    \caption{\textbf{Effects of the number of unfolded hands on the BH.}}
    \label{reb_tab:efficiency}
    \vspace{-4mm}
\end{table}
